# Supplementary material for: LUMix: Improving Mixup by Better Modelling Label Uncertainty
Source: arXiv:2211.15846 source file (2022-11-29)
Supplement: Supplementary file 1 [file fig_appendix_viz.tex]

\begin{figure}[!tbp]
\centering
\includegraphics[width=\linewidth]{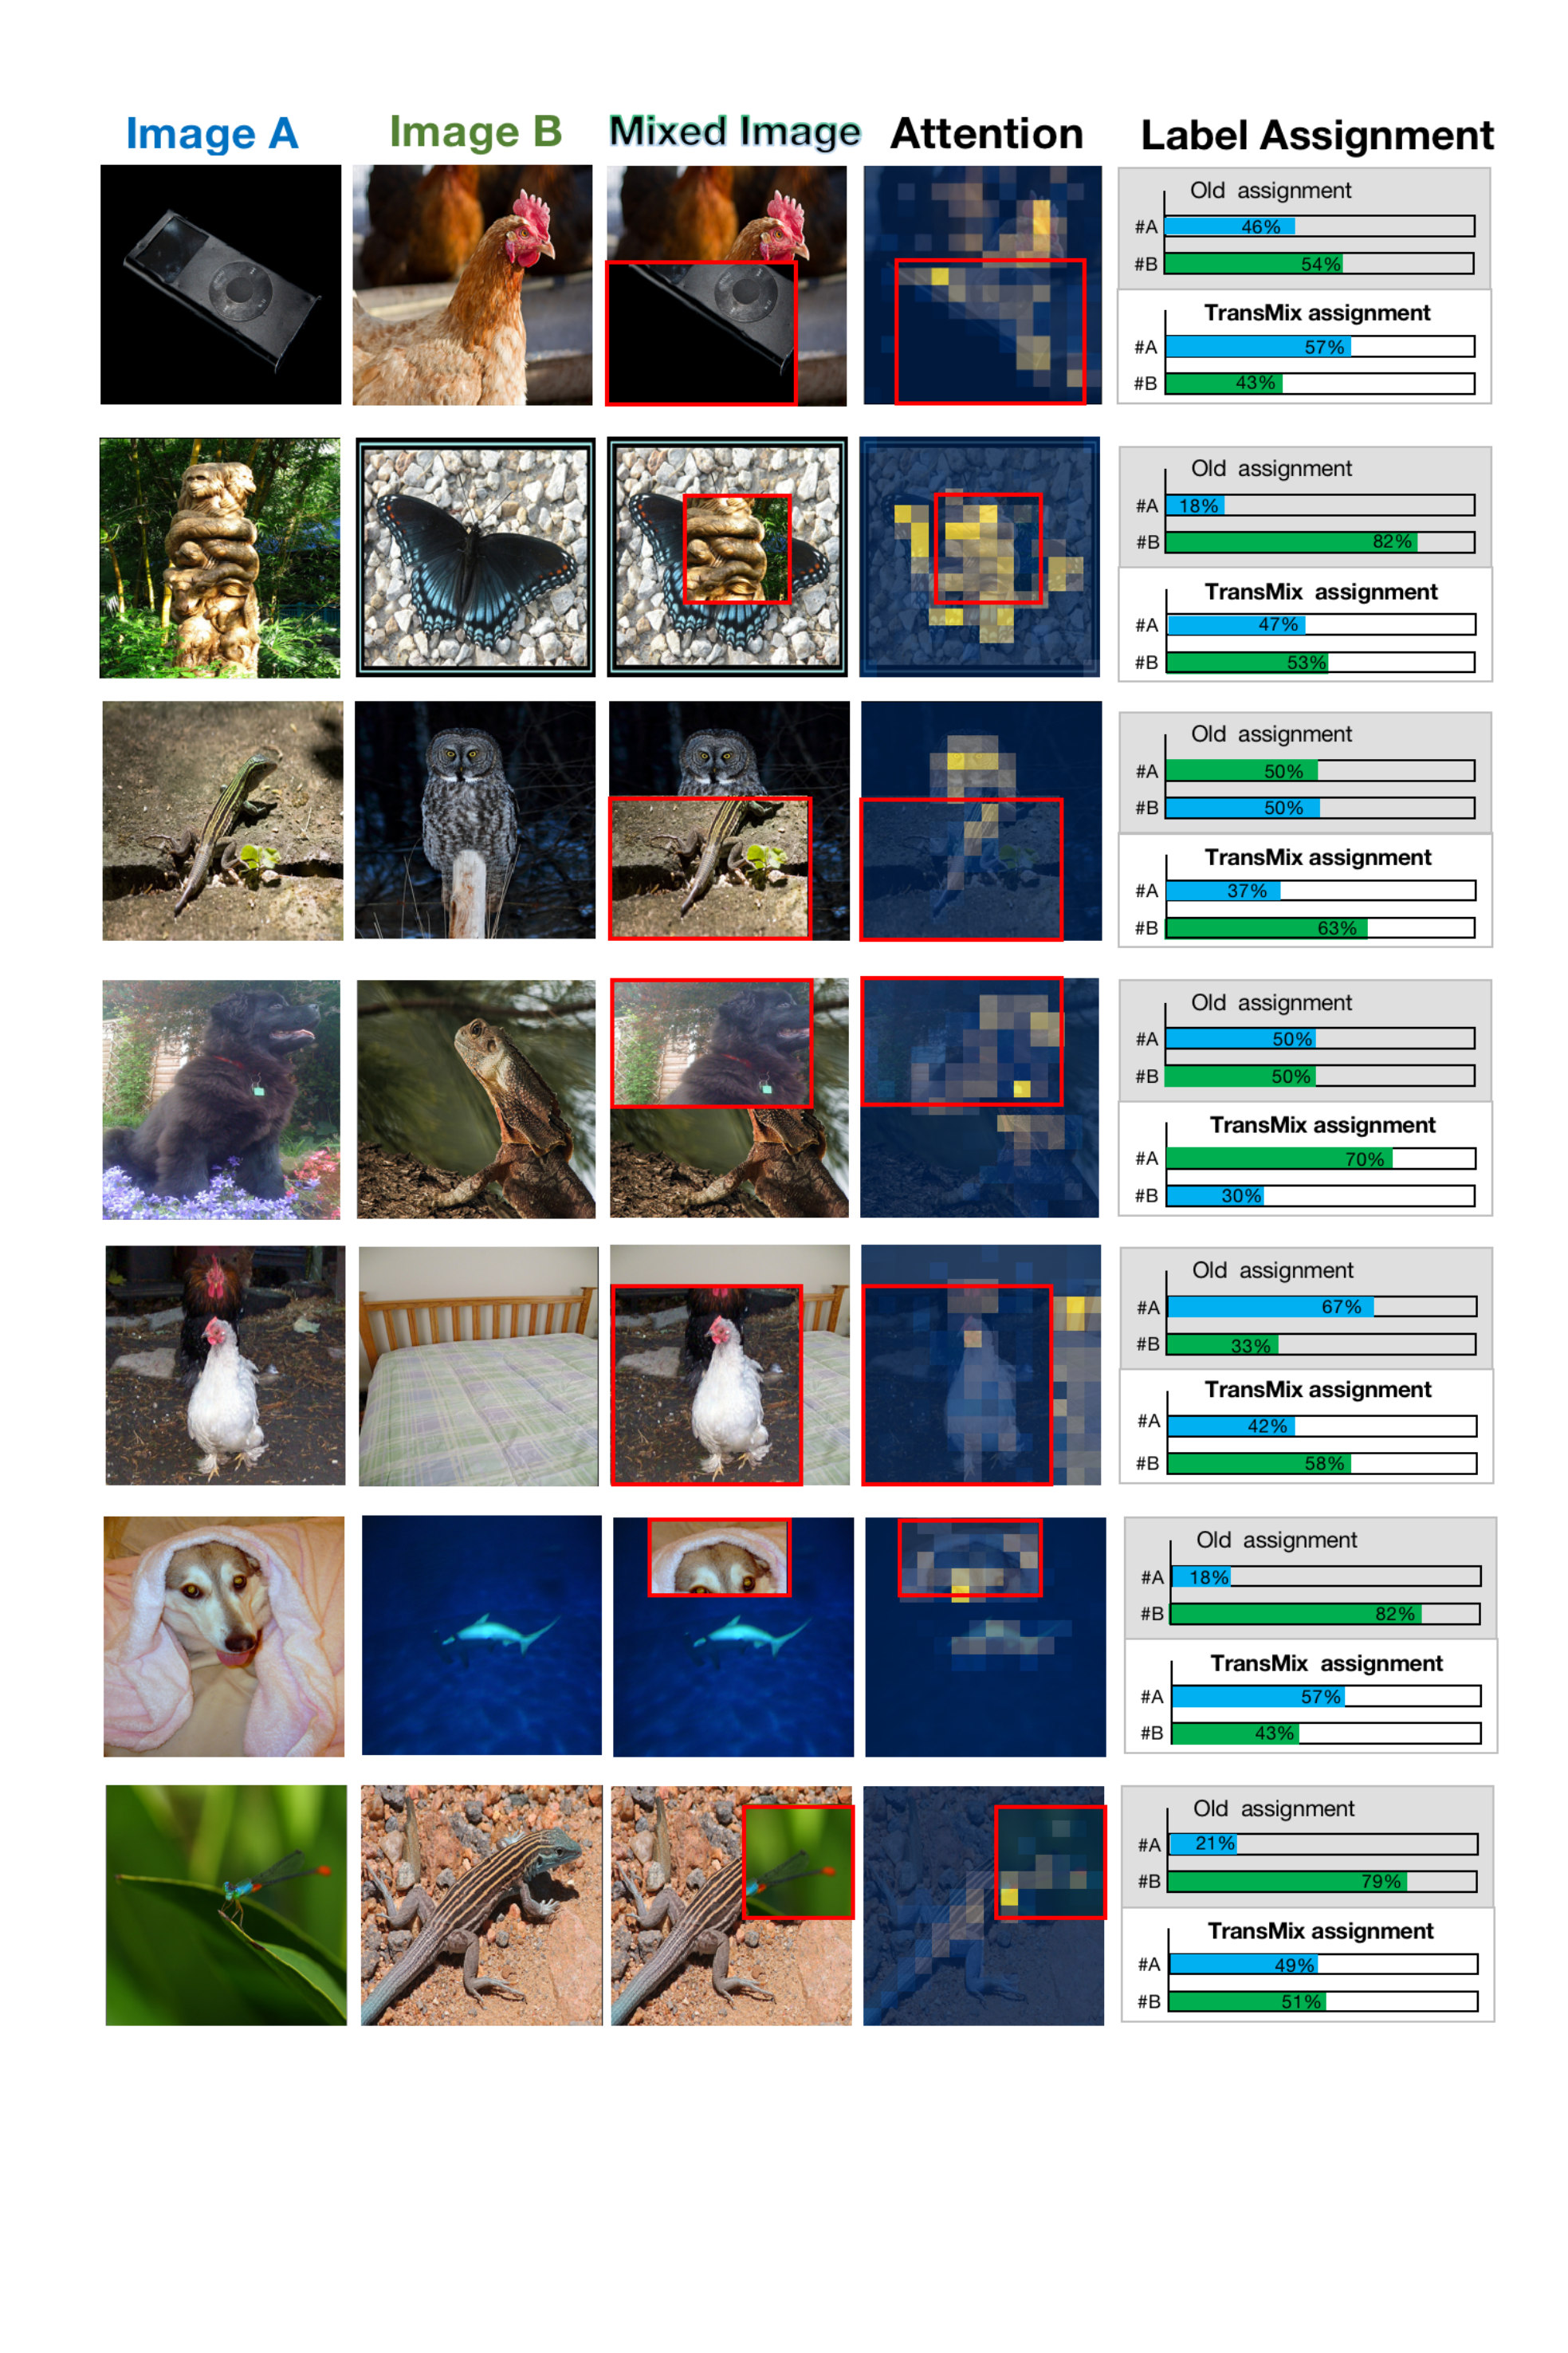}
%\vspace{-0.4cm}
\caption{The visualization including image A, image B, mixed image, attention map obtained from XCiT-L when input mixed image, and corresponding label assignments. The label assignments include both the old area-ratio assignment and new TransMix assignment. }
\label{app:fig:viz}
%\vspace{-0.1cm}
\end{figure}
