# Supplementary material for: LUMix: Improving Mixup by Better Modelling Label Uncertainty
Source: arXiv:2211.15846 source file (2022-11-29)
Supplement: Supplementary file 2 [file tab_appendix_ablation.tex]

\begin{table}[t]
\tablestyle{2pt}{1.3}
\begin{tabular}{ccccccccc}
\hline
$d$ &  6    & 8  & 10  & 12  & rollout \\
\hline
top-1 Acc & 80.3 &  80.3 & 80.4 & 80.7 &  80.4 \\
\hline
\end{tabular}
\vspace{3pt}
\caption{\textbf{Ablation study} on attention generation. Attention matrix used for TransMix is output from the $d$-th block of DeiT-S. Following~\cite{abnar-quantifying, Chefer_2021_CVPR}, rollout applies matrix multiplication across all 12 blocks' attention matrices.}
\end{table}
