# Supplementary material for: LUMix: Improving Mixup by Better Modelling Label Uncertainty
Source: arXiv:2211.15846 source file (2022-11-29)
Supplement: Supplementary file 3 [file tab_appendix_sota.tex]

\begin{table}[t]
\tablestyle{0.8pt}{1.3}
\begin{tabular}{ccccc}
\toprule[1.5pt]
Method & Backbone & Params &  top-1 Acc (\%) \\
\hline
Baseline & \multirow{4}{*}{ResNet-50} &  25M  &   76.3 \\
CutMix~\cite{yun2019cutmix} & &  25M  &  78.6  \\
SaliencyMix~\cite{uddin2020saliencymix} &  &  25M  &   78.7  \\
Puzzle-Mix~\cite{kim2020puzzle} &  &  25M  & 78.8 \\

\hline
Baseline & \multirow{6}{*}{DeiT-S} &  22M  &   78.6 \\
CutMix~\cite{yun2019cutmix} & &  22M  &  79.8 \\
% params: 22.1+23.5; flops: 4.14
Attentive-CutMix~\cite{walawalkar2020attentive} &  & 46M  &    77.5 \\
SaliencyMix~\cite{uddin2020saliencymix} &  &  22M  &   79.2  \\
Puzzle-Mix~\cite{kim2020puzzle} &  &  22M  &   79.8  \\
TransMix & &  22M &   80.7 \\
\bottomrule[1.5pt]
\end{tabular}
\vspace{3pt}
\caption{  Comparison with state-of-the-art Mixup variants with the backbone of either ViT or CNN on ImageNet-1k. All listed models are trained for 300 epochs towards fair comparison. ResNet-50 results are borrowed from the paper~\cite{uddin2020saliencymix}.}

\label{tab:sota-cnn}
\end{table}
